# Supplementary material for: What Lies Beneath? Exploring the Impact of Underlying AI Model Updates in AI-Infused Systems
Source: arXiv:2311.10652 source file (2025-03-03)
Supplement: Supplementary file 1 [file study_1_model_output.tex]

\section{Mixed Effects Model Outputs}
\label{appendix:mixed_effects_models}

\subsection{Distinguishing Models: Perceived Accuracy vs. Objective Characteristics}\label{appendix:findings_h2}

We include the detailed output of the generalized linear mixed effects model used to examine whether participants relied on observable model characteristics (e.g., latency, result count) or their own perceived accuracy to distinguish between models. This analysis corresponds to Section~\ref{sec:findings_h2} in the main text.

\begin{verbatim}
Generalized linear mixed model fit by maximum likelihood (Laplace Approximation) ['glmerMod']
Family: binomial  ( logit )
Formula: user_model_comparison_binary ~ latency_diff_scaled + result_count_diff_scaled +      perceived_accuracy_diff_scaled + (1 | session_id)
   Data: df

     AIC      BIC   logLik deviance df.resid 
  2159.2   2186.5  -1074.6   2149.2     1752 

Scaled residuals: 
    Min      1Q  Median      3Q     Max 
-1.7272 -0.7875 -0.3763  0.8605  6.2023 

Random effects:
 Groups     Name        Variance Std.Dev.
 session_id (Intercept) 0.4657   0.6825  
Number of obs: 1757, groups:  session_id, 252

Fixed effects:
                               Estimate Std. Error z value Pr(>|z|)    
(Intercept)                    -0.47974    0.07086  -6.770 1.29e-11 ***
latency_diff_scaled             0.06054    0.06022   1.005    0.315    
result_count_diff_scaled        0.03753    0.05908   0.635    0.525    
perceived_accuracy_diff_scaled -0.89630    0.07394 -12.122  < 2e-16 ***
---
Signif. codes:  0 ‘***’ 0.001 ‘**’ 0.01 ‘*’ 0.05 ‘.’ 0.1 ‘ ’ 1

Correlation of Fixed Effects:
            (Intr) ltnc__ rsl___
ltncy_dff_s -0.005              
rslt_cnt_d_  0.003 -0.321       
prcvd_ccr__  0.222 -0.027  0.059
\end{verbatim}

\subsection{Factors influencing Perceived Accuracy}

We include the detailed output of the generalized linear mixed effects model used to examine which factors influenced the perceived accuracy of a given model. This analysis corresponds to Section~\ref{sec:findings_perceived_accuracy_factors} in the main text.

\begin{verbatim}
Linear mixed model fit by REML. t-tests use Satterthwaite's method ['lmerModLmerTest']
Formula: perceived_accuracy ~ facial_match_count + rep_match_count + ns_count +      diff_count + search_results_count + model_type + overall_timer +  
    seen_tiles + mean_target_comparison_time + latency + (1 |      session_id) + (1 | task_id)
   Data: df

REML criterion at convergence: 20852.3

Scaled residuals: 
    Min      1Q  Median      3Q     Max 
-5.2073 -0.4940  0.1214  0.6061  5.3309 

Random effects:
 Groups     Name        Variance Std.Dev.
 session_id (Intercept)  555.61  23.571  
 task_id    (Intercept)   24.96   4.996  
 Residual               1554.75  39.430  
Number of obs: 2016, groups:  session_id, 252; task_id, 8

Fixed effects:
                             Estimate Std. Error        df t value Pr(>|t|)    
(Intercept)                   19.1127     2.7291   21.9115   7.003 5.10e-07 ***
facial_match_count            23.5355     1.0502 1998.9006  22.411  < 2e-16 ***
rep_match_count               16.6758     1.0244 1984.1011  16.279  < 2e-16 ***
ns_count                       2.9388     1.0867 2000.0761   2.704 0.006902 ** 
diff_count                    -7.0787     1.5766 1906.5875  -4.490 7.55e-06 ***
search_results_count           5.9723     1.2112 1884.9401   4.931 8.91e-07 ***
model_typerecognition_04      14.2293     2.3095 1842.6505   6.161 8.84e-10 ***
overall_timer                 -6.2852     2.0136 1505.9057  -3.121 0.001834 ** 
seen_tiles                    -4.7527     1.2930 1976.4139  -3.676 0.000244 ***
mean_target_comparison_time    9.6421     1.4457 1931.4743   6.669 3.34e-11 ***
latency                        0.3769     1.0954 2000.2490   0.344 0.730837    
---
Signif. codes:  0 ‘***’ 0.001 ‘**’ 0.01 ‘*’ 0.05 ‘.’ 0.1 ‘ ’ 1

Correlation of Fixed Effects:
            (Intr) fcl_m_ rp_mt_ ns_cnt dff_cn srch__ md__04 ovrll_ sn_tls mn_t__
fcl_mtch_cn  0.051                                                               
rp_mtch_cnt  0.035  0.074                                                        
ns_count     0.036  0.056  0.106                                                 
diff_count   0.015  0.121 -0.042  0.006                                          
srch_rslts_ -0.223 -0.070 -0.072 -0.099  0.004                                   
mdl_typr_04 -0.426 -0.119 -0.083 -0.084 -0.036  0.524                            
overall_tmr -0.007 -0.183 -0.144 -0.262 -0.647  0.042  0.016                     
seen_tiles  -0.073  0.025  0.040  0.010 -0.139 -0.097  0.172 -0.335              
mn_trgt_cm_  0.019  0.119  0.096  0.087  0.414 -0.072 -0.044 -0.552  0.195       
latency     -0.002  0.010  0.024  0.045  0.110 -0.313  0.006 -0.162  0.008  0.070
\end{verbatim}

\subsection{Factors influencing model preference}

We include the detailed output of the logistic regression model used to analyze the factors influencing participants' preferences between Model A-UP and Model B-UP. The analysis evaluates the effects of trial count, match findings, and perceived accuracy on model preference, discussed in Section~\ref{sec:model_preference}. The significant predictors are highlighted in the output below.

\begin{verbatim}
glm(formula = preferred_model_binary ~ model_A_trial_count + 
model_A_trial_count_match_found + model_A_avg_perceived_accuracy + 
model_B_trial_count_match_found + model_B_avg_perceived_accuracy, 
family = binomial(link = "logit"), data = df)

Coefficients:
                                 Estimate Std. Error z value Pr(>|z|)    
(Intercept)                      0.400568   1.327662   0.302    0.763    
model_A_trial_count             -0.308623   0.299720  -1.030    0.303    
model_A_trial_count_match_found  0.075469   0.189530   0.398    0.690    
model_A_avg_perceived_accuracy  -0.033977   0.006874  -4.942 7.71e-07 ***
model_B_trial_count_match_found  0.092030   0.190740   0.482    0.629    
model_B_avg_perceived_accuracy   0.037990   0.006681   5.686 1.30e-08 ***
---
Signif. codes:  0 ‘***’ 0.001 ‘**’ 0.01 ‘*’ 0.05 ‘.’ 0.1 ‘ ’ 1

(Dispersion parameter for binomial family taken to be 1)

    Null deviance: 321.43  on 240  degrees of freedom
Residual deviance: 225.78  on 235  degrees of freedom
  (11 observations deleted due to missingness)
AIC: 237.78

Number of Fisher Scoring iterations: 5
\end{verbatim}

\subsection{Impact of the underlying model on the comparison decisions}

We include the detailed output of the generalized linear mixed effects model used to examine the impact of the underlying model on the comparison decisions. This analysis corresponds to Section~\ref{sec:findings_h5} in the main text.

These are the outputs for the three models: positive vs. rest, negative vs. rest, and uncertain vs. rest.

\begin{verbatim}
Generalized linear mixed model fit by maximum likelihood (Laplace Approximation) ['glmerMod']
Family: binomial  ( logit )
Formula: positive_vs_rest ~ model_type + (1 | session_id)
Data: df

 AIC      BIC   logLik deviance df.resid 
11472.1  11493.9  -5733.0  11466.1    10643 

Scaled residuals: 
Min      1Q  Median      3Q     Max 
-2.1231 -0.6113 -0.4218  0.7908  5.4912 

Random effects:
Groups     Name        Variance Std.Dev.
session_id (Intercept) 0.8151   0.9028  
Number of obs: 10646, groups:  session_id, 252

Fixed effects:
                     Estimate Std. Error z value Pr(>|z|)    
(Intercept)              -1.01287    0.06717 -15.080  < 2e-16 ***
model_typerecognition_04  0.38091    0.04906   7.764 8.21e-15 ***
---
Signif. codes:  0 ‘***’ 0.001 ‘**’ 0.01 ‘*’ 0.05 ‘.’ 0.1 ‘ ’ 1

Correlation of Fixed Effects:
        (Intr)
mdl_typr_04 -0.378

\end{verbatim}

\begin{verbatim}
Generalized linear mixed model fit by maximum likelihood (Laplace Approximation) ['glmerMod']
Family: binomial  ( logit )
Formula: negative_vs_rest ~ model_type + (1 | session_id)
Data: df

 AIC      BIC   logLik deviance df.resid 
13100.2  13122.0  -6547.1  13094.2    10643 

Scaled residuals: 
Min      1Q  Median      3Q     Max 
-3.6717 -0.8580  0.4317  0.7729  3.0907 

Random effects:
Groups     Name        Variance Std.Dev.
session_id (Intercept) 0.8162   0.9034  
Number of obs: 10646, groups:  session_id, 252

Fixed effects:
                     Estimate Std. Error z value Pr(>|z|)    
(Intercept)               0.18270    0.06562   2.784  0.00537 ** 
model_typerecognition_04 -0.36777    0.04533  -8.113 4.92e-16 ***
---
Signif. codes:  0 ‘***’ 0.001 ‘**’ 0.01 ‘*’ 0.05 ‘.’ 0.1 ‘ ’ 1

Correlation of Fixed Effects:
        (Intr)
mdl_typr_04 -0.338
\end{verbatim}

\begin{verbatim}
Generalized linear mixed model fit by maximum likelihood (Laplace Approximation) ['glmerMod']
 Family: binomial  ( logit )
Formula: uncertain_vs_rest ~ model_type + (1 | session_id)
   Data: df

     AIC      BIC   logLik deviance df.resid 
  8750.3   8772.1  -4372.1   8744.3    10643 

Scaled residuals: 
    Min      1Q  Median      3Q     Max 
-0.9543 -0.4570 -0.3581 -0.2578  4.9061 

Random effects:
 Groups     Name        Variance Std.Dev.
 session_id (Intercept) 0.5016   0.7082  
Number of obs: 10646, groups:  session_id, 252

Fixed effects:
                         Estimate Std. Error z value Pr(>|z|)    
(Intercept)              -1.81609    0.06201 -29.287   <2e-16 ***
model_typerecognition_04  0.08289    0.05790   1.432    0.152    
---
Signif. codes:  0 ‘***’ 0.001 ‘**’ 0.01 ‘*’ 0.05 ‘.’ 0.1 ‘ ’ 1

Correlation of Fixed Effects:
            (Intr)
mdl_typr_04 -0.465    
\end{verbatim}

\subsection{Impact of Model Type on Search Behavior}

We include the detailed output of the linear mixed effects models used to examine the impact of the underlying model on the search behavior, specifically on the number of comparisons made, the time spent on the search results page, and the number of results checked. This analysis corresponds to Section~\ref{sec:findings_h5} in the main text.

\begin{verbatim}
Linear mixed model fit by REML. t-tests use Satterthwaite's method ['lmerModLmerTest']
Formula: total_num_comparisons ~ model_type + (1 | session_id)
   Data: df

REML criterion at convergence: 14139.9

Scaled residuals: 
    Min      1Q  Median      3Q     Max 
-2.0686 -0.1943 -0.0892 -0.0029 20.8738 

Random effects:
 Groups     Name        Variance Std.Dev.
 session_id (Intercept)  8.64    2.939   
 Residual               59.12    7.689   
Number of obs: 2016, groups:  session_id, 252

Fixed effects:
                          Estimate Std. Error        df t value Pr(>|t|)    
(Intercept)                 5.7866     0.3079  518.8372  18.791  < 2e-16 ***
model_typerecognition_04   -1.0048     0.3509 1896.8430  -2.863  0.00424 ** 
---
Signif. codes:  0 ‘***’ 0.001 ‘**’ 0.01 ‘*’ 0.05 ‘.’ 0.1 ‘ ’ 1

Correlation of Fixed Effects:
            (Intr)
mdl_typr_04 -0.574
\end{verbatim}

\begin{verbatim}
Linear mixed model fit by REML. t-tests use Satterthwaite's method ['lmerModLmerTest']
Formula: overall_timer ~ model_type + (1 | session_id)
Data: df

REML criterion at convergence: 23280.3

Scaled residuals: 
Min      1Q  Median      3Q     Max 
-2.7329 -0.4519 -0.1463  0.2863 18.4644 

Random effects:
Groups     Name        Variance Std.Dev.
session_id (Intercept) 1510     38.86   
Residual               5248     72.44   
Number of obs: 2016, groups:  session_id, 252

Fixed effects:
                     Estimate Std. Error       df t value Pr(>|t|)    
(Intercept)               125.079      3.378  427.941  37.032  < 2e-16 ***
model_typerecognition_04  -16.744      3.331 1856.454  -5.027 5.46e-07 ***
---
Signif. codes:  0 ‘***’ 0.001 ‘**’ 0.01 ‘*’ 0.05 ‘.’ 0.1 ‘ ’ 1

Correlation of Fixed Effects:
        (Intr)
mdl_typr_04 -0.497
\end{verbatim}

\begin{verbatim}
Linear mixed model fit by REML. t-tests use Satterthwaite's method ['lmerModLmerTest']
Formula: seen_tiles ~ model_type + (1 | session_id)
   Data: df

REML criterion at convergence: 17784.4

Scaled residuals: 
    Min      1Q  Median      3Q     Max 
-1.9846 -0.4864 -0.0937  0.1384 13.1841 

Random effects:
 Groups     Name        Variance Std.Dev.
 session_id (Intercept)  53.69    7.327  
 Residual               360.65   18.991  
Number of obs: 2016, groups:  session_id, 252

Fixed effects:
                          Estimate Std. Error        df t value Pr(>|t|)    
(Intercept)                21.0858     0.7632  516.8290   27.63   <2e-16 ***
model_typerecognition_04  -11.5951     0.8669 1895.9167  -13.38   <2e-16 ***
---
Signif. codes:  0 ‘***’ 0.001 ‘**’ 0.01 ‘*’ 0.05 ‘.’ 0.1 ‘ ’ 1

Correlation of Fixed Effects:
            (Intr)
mdl_typr_04 -0.572    
\end{verbatim}
